# Supplementary material for: On the Stability-Plasticity Dilemma of Class-Incremental Learning
Source: arXiv:2304.01663 source file (2023-04-04)
Supplement: Supplementary file 1 [file appendix.tex]

\begin{itemize}
    \item mini-batch CKA
    \item CKA experimental settings (flatten feature maps for $p_1$ and $p_2$)
\end{itemize}
